# Supplementary material for: MaxRay: A Raytracing-based Integrated Sensing and Communication Framework
Source: arXiv:2112.01751 source file (2021-12-03)
Supplement: Supplementary file 1 [file appendix.tex]

\section{Appendix}
